# Supplementary material for: Meta-Learning of NAS for Few-shot Learning in Medical Image Applications
Source: arXiv:2203.08951 source file (2022-03-16)
Supplement: Supplementary file 1 [file appendix01.tex]

\begin{frontmatter}
\chapter{Appendix title}%\label{chap:appa}
\end{frontmatter}

%\section{}\label{}
