# Supplementary material for: Meta-Learning of NAS for Few-shot Learning in Medical Image Applications
Source: arXiv:2203.08951 source file (2022-03-16)
Supplement: Supplementary file 2 [file appendix02.tex]

\begin{frontmatter}
\chapter{Appendix title}%\label{chap:appb}
\end{frontmatter}
